# Supplementary material for: Test-time Controllable Image Generation by Explicit Spatial Constraint Enforcement
Source: arXiv:2501.01368 source file (2025-01-02)
Supplement: Supplementary file 1 [file Andrew.tex]

\begin{algorithm}[tb]
    \caption{Andrew convex hull algorithm}
    \label{alg:Andrew}
    \textbf{Input}: pixel coordinate set $p$\\
    \textbf{Output}: coordinate set $convexhull$ \\
    \begin{algorithmic}[1] %[1] enables line numbers
        \STATE sort $p$
        \STATE empty vertex vector $vt$
        \STATE $vt\ \leftarrow \ p_1$
        \FOR{ $i = 2$ \textbf{ to } $size(p)$ }
            \WHILE{$(vt_{-1}-vt_{-2}])$  $ \ \times \ (p[i] - vt_{-1})<= 0)$}
            \STATE \textbf{delete} $vt_{-1}$
            \ENDWHILE
            \STATE $vt\ \leftarrow \ p_i$
        \ENDFOR
        \FOR{ $i = size(p) - 1$ \textbf{ down to } $1$ }
            \WHILE{$(vt_{-1}-vt_{-2}])$  $ \ \times \ (p[i] - vt_{-1})<= 0)$}
            \STATE \textbf{delete} $vertex_{-1}$
            \ENDWHILE
            \STATE $vt\ \leftarrow \ p_i$
        \ENDFOR
        \STATE convert vertex vector $vt$ to pixel set $convexhull$
        \STATE \textbf{return} $convexhull$
    \end{algorithmic}
\end{algorithm}
